# Supplementary material for: Cooperative Protocols for Random Access Networks
Source: arXiv:0808.3502 source file (2009-01-23)
Supplement: Supplementary file 1 [file appendix.tex]

\section{Achievable Rate for Decode Forward}
\label{app:decodeForward}
We provide an argument why \eqref{eq:rateDecodeForward} is achievable.
